# Supplementary material for: Brick-DICL: Dynamic In-Context Learning for Automated Brick Schema Classification
Source: arXiv:2606.17637 source file (2026-06-16)
Supplement: Supplementary file 1 [file appendix.tex]

% \setcounter{section}{0}
% \section*{Appendix}
\appendix
\textbf{\huge{Appendix}}
\section{Pseudo-code}
This section shows the pseudo-code of Brick-DICL, which includes two main modules: two stage DICL, and multi-LLM for low-confidence generation filter.~\label{code}
\begin{algorithm}[h]

\caption{Brick-DICL Classification Pipeline}\label{alg:code}
\begin{algorithmic}[1]
    \REQUIRE{BMS point data $\mathcal{D}$, Brick classes $\mathcal{C}$, LLMs $\mathcal{M}$, Training examples $\mathcal{T}$}
    \ENSURE{Classified BMS points with Brick classes $\{(p_i, c_{\text{final}})\}$}
    
    \STATE \textbf{Data Standardization:}
    \FOR{each $p \in \mathcal{D}$}
        \STATE Normalize metadata attributes: equipment type, point type, units, markers
        \STATE Generate missing descriptions using $\mathcal{M}_{\text{desc}}$
    \ENDFOR
    
    \STATE \textbf{Build RAG Databases:}
    \STATE Meta-data RAG: Create embedding vectors for training examples
    \STATE Class RAG: Create embedding vectors for Brick class definitions
    
    \textbf{\textit{Classification Process}:}
    \FOR{each BMS point $p_i \in \mathcal{D}$}
        \STATE \textbf{Stage One - Metadata ICL:}
        \STATE Retrieve top-$k$ similar examples from Meta-data RAG
        \STATE Construct dynamic prompt with examples and input attributes
        \STATE Generate initial Brick class prediction $c_{\text{brick}}^{(1)}$
        
        \STATE \textbf{Stage Two - Class ICL:}
        \STATE Retrieve top-$m$ relevant classes from Class RAG
        \STATE Construct refinement prompt with class definitions
        \STATE Generate top-3 predictions $\{(c_1,p_1),(c_2,p_2),(c_3,p_3)\}$
        
        \STATE \textbf{Multi-LLM Filtering:}
        \FOR{each LLM $M_j \in \mathcal{M}$}
            \STATE Get predictions $(c_{\text{brick},j}^{(1)}, \{c_{1,j},c_{2,j},c_{3,j}\})$
        \ENDFOR
        \STATE Apply filtering strategies (All/Top3/Top1/Any2)
        \IF{low-confidence flagged}
            \STATE Route to human validation interface
        \ENDIF
    \ENDFOR
    
    \textbf{\textit{Human Validation}:}
    \FOR{each flagged prediction}
        \STATE Present multi-LLM predictions and justifications
        \STATE Store expert-validated results
    \ENDFOR
    
    \STATE \textbf{Return} Final classifications with confidence scores
\end{algorithmic}~\label{alg: code}
\end{algorithm}

\newpage
\section{Prompting Techniques}
\subsection{Prompting for Stage One Metadata DICL}
~\label{sec: stage1prompt}
 \vspace{-0.2in}
 \begin{lstlisting}[caption=Prompting of Stage One Dynamic In-context Learning for Point Brick Prediction.]
#  user prompt
prompt = """
You are an AI assistant specialized in Brick schema classification. Your task is to analyze building equipment and point data, then map them to appropriate Brick schema classes.

Input:
You will receive a set of attributes describing building equipment and associated data points. These attributes may include: equipment type name, equipment description, equipment markers, point type name, point description, point function, point markers, point keywords, possible point class, unit of measurement (UoM), data type, and facets.
Note: Some attributes may be missing in the input.

Examples:
{retrieved_examples}

These above examples show how various attribute combinations map to specific Brick classes. Use them as reference for your predictions.

Your Task:
1.  Analyze the given attributes for the equipment and point.
2. Compare the input to the provided examples.
3. Predict the most appropriate Brick class for both the equipment and the point.
4. Provide a justification for your predictions.
5. Assign a confidence score (1-10) to your predictions.

Output Format:
Please STRICTLY adhere to the following format for your response:

<Response>
Equipment Brick Class: <Predicted class, e.g., RTU, GM, WM, DCA>
Point Brick Class: <Predicted class>
Justification: <Your reasoning for both predictions>
Confidence: <Score from 1-10>
</Response>

Input for Classification:
{sample_attributes}

Please provide your classification and reasoning based on the given input, following the specified output format.

"""

\end{lstlisting}

\newpage
\subsection{Prompting for Stage Two Class DICL}
~\label{sec: stage2prompt}
\vspace{-0.2in}
\begin{lstlisting}[caption=Prompting of Stage Two In-context Learning for Point Brick Classification.]
#  user prompt
prompt = """
You are an AI assistant specialized in Brick schema classification for building equipment and data points. Your task is to analyze the given attributes and map them to appropriate Brick schema classes, with a specific focus on selecting the top 3 point Brick classes from a provided list.

Input:
You will receive a set of attributes describing building equipment and associated data points. These attributes may include: equipment type name, equipment description, equipment markers, point type name, point description, point function, point markers, point keywords, possible point class, unit of measurement (UoM), data type, and facets.
Note: Some attributes may be missing in the input.

Brick Class List:
The following is a focused subset of Brick classes. You MUST select the Point Brick Class from this list:
{retrieved_brick_classes}

Examples:
{retrieved_examples}

These examples demonstrate how various attribute combinations map to specific Brick classes. Use them as a reference for your predictions.

Your Task:
1. Analyze the given attributes for the equipment and point.
2. Compare the input to the provided examples.
3. From the provided Brick Class List, select the 5 most likely classes for the point.
4. For each of the 5 classes, provide reasons why it could be the best answer and why it might not be.
5. Choose the top 3 classes that you think are the best match for the point.
6. Assign a probability between 0 and 1 for each of the top 3 classes. The sum of these probabilities must equal 1.
Provide a justification for your predictions.

Output Format:
Please STRICTLY adhere to the following format for your response:

<Response>
Equipment Brick Class: <Predicted class, e.g., RTU, GM, WM, DCA>
Point Brick Class: <[Class 1], [Probability 1], [Class 2], [Probability 2], [Class 3], [Probability 3]>
Justification: <Your reasoning for these classifications>
Confidence: <Score from 1-10>
</Response>

Input for Classification:
{sample_attributes}

Please analyze the given attributes, refer to the provided examples, and predict the Equipment Brick Class and top 3 Point Brick Classes based on this information. Ensure that your Point Brick Class predictions come from the provided Brick Class List. Follow the specified output format precisely.

"""
\end{lstlisting}
